# Supplementary material for: Action-conditioned video data improves predictability
Source: arXiv:2404.05439 source file (2024-04-08)
Supplement: Supplementary file 1 [file X_suppl.tex]

\clearpage
\setcounter{page}{1}
\maketitlesupplementary

\section{Adversarial Loss}
In addition to the reconstruction penalty discussed in \textit{Sec. 2.3: Loss and Training Loop} of the paper, we also use the adversarial loss given in \cite{mathieu}, \cite{villegas} and \cite{sarkar2021} to increase the sharpness of the generated images. In general, deterministic frameworks (like ACVG, ACPNet or MCNet) suffer from the averaging effects of the convolution operations and are compensated by adding the adversarial loss. The expression for the adversarial loss $\mathcal{L}_{adv}$ is similar to \cite{mathieu},:
\begin{equation}
 \mathcal{L}_{adv}=-\text{log}\sD([{x}_{-n+1:0},\tx_{1:T}]) \label{eq:L_adv}  
\end{equation}
where ${x}_{-n+1:0}$ is the sequence of n past input images,  $\tx_{1:T}$ represents the predicted future images by the generator of ACVG given by Eqs. (11) or (12) depending upon the generator or dual training phase of the network, and $\sD(.)$ is the output from the discriminator network. Let $x_{-n+1:T}$ be the concatenation of all $n+T$ ground truth images. The discriminator network is trained  on the loss function: 
\begin{equation}
    \mathcal{L}_{dis}=-\text{log}\sD(x_{-n+1:T})-\text{log}(1-\sD({x}_{-n+1:0},\tx_{1:T}))
\end{equation}
 The adversarial loss $\mathcal{L}_{adv}$ is scaled by a factor of $\mu $ before being added to the total reconstruction loss of the Generator Network given by Eqs. (20) and  (21) in the paper. The scaling factor $\mu$ is chosen to be much less than 1. In the case of RoAM dataset,  we choose $\mu=0.0001$.

 \section{Architecture of the network}\label{sup_sec:Net_architecture} 
 Given that the objective of this paper is to show with extensive empirical study that incorporating the action of the recording platform into the video prediction framework can significantly improve the quality of the predicted image frames, we have kept the general architecture of the Generator of ACVG is kept similar to that of the basic architecture of MCNet \cite{villegas}. The Encoder modules are denoted by $\Theta^{\enc}_G$ in Fig. 2a and described in \textit{Sec. 2.1: Generator Network} of the paper, is designed with 3 stacked layers of Convolutional neural networks \cite{cnn} followed by a max-pooling layer \cite{imagenet}. Both the encoder modules for the image as well as the flow map (\textit{Fig. 2a}) follow this same architectural design. We use a single layer of Convolutional LSTM \cite{convlstm} cells to design the recurrent module, $\Theta^{r}_G$  of the Generator (\textit{Fig. 2a} in the paper). The decoder module $\Theta^{\dec}_G$ is designed as the inversion operation to the convolution operations in the encoder module and is designed with stacked layers of 2D upsampling layers followed by deconvolution or 2D transpose convolutional layers similar to \cite{villegas,sarkar2021,acpnet2023}. We employ a similar architecture for the residual module illustrated by the blue shaded box in Figure 2a of the paper from the work of Villegas \cite{villegas}. 

We use a single LSTM layer \cite{lstm} with  2 cell units (since the dimension of the action space of the recording agent is 2 here) to design the recurrent module $\Theta^r_A$ of the Actor-network of ACVG (\textit{Fig. 2b} in the paper). In order to approximate the future action at time-step $t+1$, we further encode the already encoded future image map  $\tilde{\chi}_{t+1}$ coming from the generator network (refer to \textit{Fig. 2b} in the paper) into a lower dimensional manifold with layers of convolutional NN and maxpooling layers. These 2-dimensional image maps are then flattened and combined with $\hat{\alpha}_t$ in the decoder module $\sF^{dec}_A$ as indicated in Eq. 15 of the paper to generate the future action $\tilde{a}_{t+1}$. The decoder module ($\Theta^{\dec}_A$) of the Actor-Network is designed with stacked layers of fully connected dense layer followed by Dropout \cite{dropout} and Batch Normalisation \cite{batchnorm} to prevent overfitting. 

The architecture of the discriminator network is the same as given in \cite{sarkar2021}. 
The codes for the implementation ACVG can be found in \url{https://github.com/Not-a-R0b0t/ACVG-CVPR24-17749-main.git}

\section{RoAM Dataset }\label{sup_sec:roam}
As described in \textit{Sec. 3: RoAM dataset and Experimental Setup} of the paper, RoAM or Robot Autonomous Motion dataset is a new video-action dataset introduced by Sarkar et al. \cite{acpnet2023}. This dataset is recorded with a Zed mini stereo camera attached to a custom-made turtlebot3 robot \cite{acpnet2023} and is the only publicly available video dataset that offers synchronised and time-stamped image frames along with the corresponding action sequences in the partially observable scenario where the camera is mounted on a moving platform. 

To the best of our knowledge, BAIR Robot Pushing Dataset \cite{ebert17} is the only other publicly available video action pair dataset in robotics. However, in the case of the BAIR robot pushing dataset, the camera is mounted on a fixed platform and is not suitable for partially observable scenarios. Also in the case of the BAIR dataset, the actions were taken by the manipulator whose motion was observed and captured by the fixed camera and these actions were completely random in nature. In the case of RoAM, the actions taken by the moving platform or the turtlebot3 robot were not random and came from an autonomous navigation module. The autonomous navigation module in the case of the RoAM dataset deployed a geometric obstacle avoidance algorithm such that the robot could move in crowded indoor spaces without collision \cite{acpnet2023}. The action profiles recorded in the RoAM dataset are smooth in nature and thus are well suited for understanding the dual dependence and relationship between the predicted image and action pair in partially observable scenarios. Currently, the RoAM dataset can be downloaded from \url{https://meenakshisarkar.github.io/Motion-Prediction-and-Planning/dataset/} \cite{acpnet2023} as TFRecord files. However, we have attached a small sample of the dataset in the supplementary file for the reference of the readers.

\section{Additional Discussion }\label{sup_sec:discussion}
\textbf{Q: How do the results with ACVG on RoAM dataset generalize to similar other partially observable scenarios?}
While we have presented our empirical performance analysis of ACVG on the RoAM dataset which was collected with a Turtlebot3 robot, we have only used the normalized action values in the training phase such that the resulting network is not limited to a particular actuator limit and can effectively generalize to other actuator ranges. This is explained in detail in \textit{Sec. 2} of the paper. Additionally, the RoAM dataset was gathered employing the TurtleBot3 robot, a widely adopted and scalable indoor robotic platform within the research community. TurtleBot3 also benefits from its extensive open-source support through the Robot Operating System (ROS) \cite{ros}. It moves using a 2 wheeled differential drive system, complemented by a caster wheel for balance. This configuration represents one of the most common actuator setups for indoor mobile platforms. Consequently, a network trained on the RoAM dataset can be readily fine-tuned to cater to the requirements of analogous indoor navigation problem scenarios.

% Furthermore, RoAM was collected using a Trutlebot3 robot which is one of the most popular and scalable indoor robot platforms in the research community with extended open-source support from ROS \cite{ros}. It uses a 2 wheeled differential drive to move along with a caster wheel for balance which is also the most common actuator configuration for indoor mobile platforms.

\textbf{Q: How will the performance of ACVG compare to other SoTA stochastic generative architectures?}
The objective of this paper is the prove with extensive empirical results that conditioning predicted image frames on the action data in the dual Generator-Actor framework like ACVG can significantly improve performance and accuracy in partially observable scenarios where the camera is moving. To that, we have used other state-of-the-art deterministic video prediction frameworks:  VANet\cite{sarkar2021}, ACPNet \cite{acpnet2023} and MCNet \cite{villegas}, and provided detailed quantitative and qualitative performance analysis that shows how incorporating action can significantly improve the predictability of the framework. We chose  VANet and ACPNet as the comparative frameworks to ACVG since all these 3 frameworks share similar optical flow-based frame generation architectures. However, in the case of VANet, it uses both first and second-order optical flow maps or pixel difference maps for video prediction, whereas all the other frameworks use only the first-order pixel difference maps in their predictions. We have shown in Fig 3 and Fig 4 of our paper that even with a smaller parametric space, ACVG can outperform VANet (VANet uses almost 1.5 times the parameters used by the Generator Network of ACVG).

We are aware that there are multiple stochastic \cite{villegasNeurIPS2019}, \cite{Denton},\cite{slrvp2020} and more recently diffusion-based video generation models \cite{tmlr_hoppe22}, \cite{ho2022diffusion} available in the literature that can outperform these deterministic prediction frameworks. However, these stochastic generative architectures employ a much larger parametric space to generate future image frames and thus, comparing their performance to ACVG would not lead to any meaningful conclusion. The primary goal of our paper is not to position ACVG as the most optimal video prediction framework. Instead, our focus is to demonstrate that, even within a straightforward deterministic framework that relies solely on first-order pixel difference maps, integrating sequences of camera movements can result in noteworthy enhancements. We have demonstrated in Fig 4c and Fig 4d of our paper that even in the presence of a bounded random perturbation of form $\mathcal{N}(0,0.2)$ in the action input, ACVG continues to outperform ACVG-fa. This removes any confusion regarding the role of the learned action values from the actor network. The incorporation of action or movement sequences into variational inference frameworks such as \cite{Denton}, \cite{slrvp2020}, poses a non-trivial challenge due to the utilization of Gaussian Priors in these frameworks for modelling the spatio-temporal dynamics of video data. However, this presents a promising avenue for future research directions.
\begin{figure*}
\centering
\subcaptionbox{\label{fig:roam_quant_vgg16}}{\includegraphics[width=0.32\textwidth,height=3.6cm]{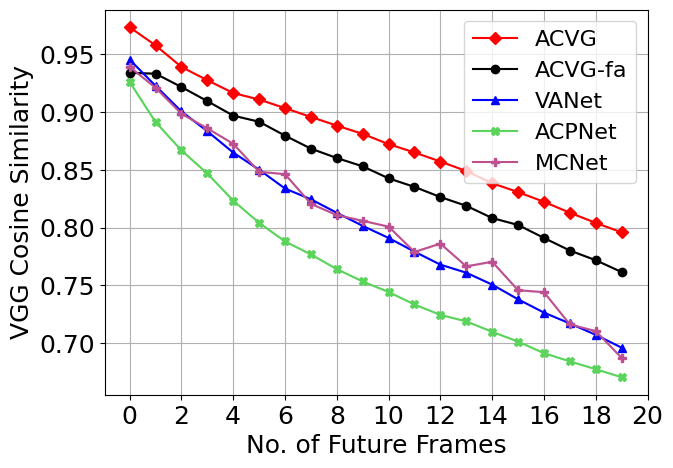}}%
\hfill % <-- Seperation
\subcaptionbox{\label{fig:roam_quant_lpips}}{\includegraphics[width=0.32\textwidth,height=3.6cm]{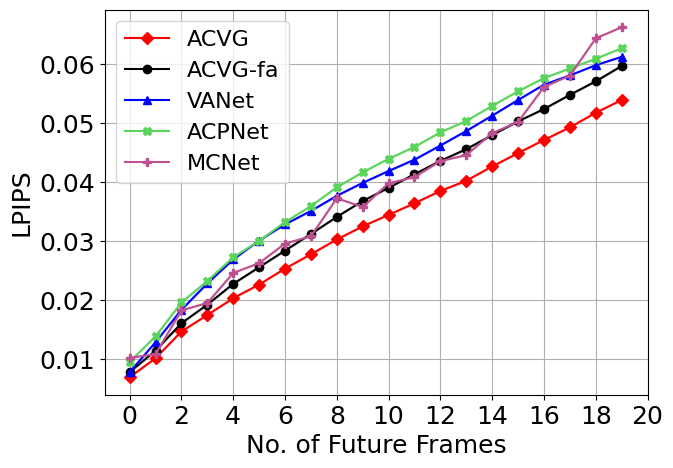}}%
\hfill % <-- Seperation
\subcaptionbox{\label{fig:roam_quant_psnr}}{\includegraphics[width=0.32\textwidth,height=3.6cm]{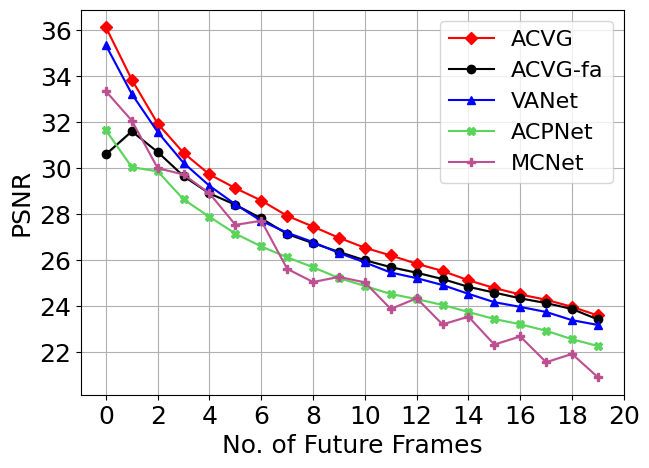}}
\caption{A Frame-wise quantitative analysis of   ACVG, ACVG-fa, ACPNet, VANet and MCNet on RoAM dataset for predicting 20 frames into the future based on the past history of 5 frames. Starting from the left, we have plotted the mean performance index for VGG 16 Cosine Similarity (\textbf{higher is better}), LPIPS score (\textbf{lower is better}), and PSNR (\textbf{higher is better}) on the test set. }
\label{fig:wacv_quant}
\end{figure*}
\begin{figure*}[ht]
\resizebox{\textwidth}{!}{\begin{tabular}{cccccccccccc}
 & t=1 & t=3 & t=5 & t=7 & t=9 & t=11 & t=13 & t=15 & t=17 & t=19\\
 GT velocity& $v=0.087$ & $v=0.088$ & $v=0.088$ & $v=0.0886$ & $v=0.089$ & $v=0.0893$ & $v=0.09$ & $v=0.0903$ & $v=0.091$ & $v=0.091$\\
Ground Truth & \imgcell{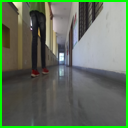} & \imgcell{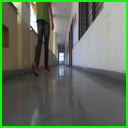} & \imgcell{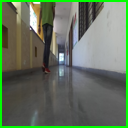}&  \imgcell{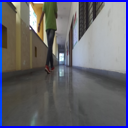}&\imgcell{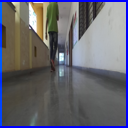} & \imgcell{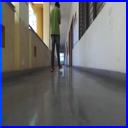} & \imgcell{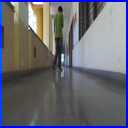} & \imgcell{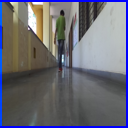} & \imgcell{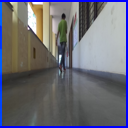} & \imgcell{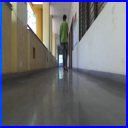} \\
&&&ACVG&  \imgcell{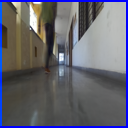}&\imgcell{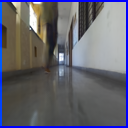} & \imgcell{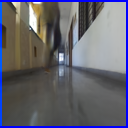} & \imgcell{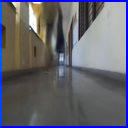} & \imgcell{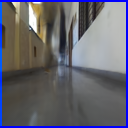} & \imgcell{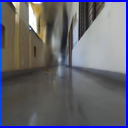} & \imgcell{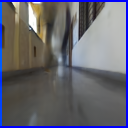} \\
&&& predicted velocity in ACVG  & $v=0.064$ & $v=0.0674$ & $v=0.073$ & $v=0.078$ & $v=0.083$ & $v=0.089$ & $v=0.093$\\
% &&& &  &&& &  &  & \\
&&&ACVG-fa&  \imgcell{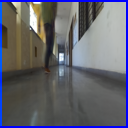}&\imgcell{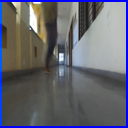} & \imgcell{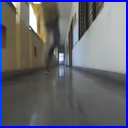} & \imgcell{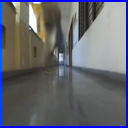} & \imgcell{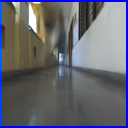} & \imgcell{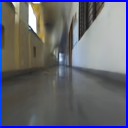} & \imgcell{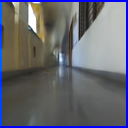}\\
&&& fixed velocity for ACVG-fa \& ACPNet  & $v=0.088$ & $v=0.088$ & $v=0.088$ & $v=0.088$ & $v=0.088$ & $v=0.088$ & $v=0.088$\\
&&&ACPNet&  \imgcell{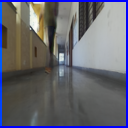}&\imgcell{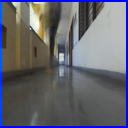} & \imgcell{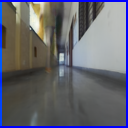} & \imgcell{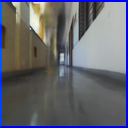} & \imgcell{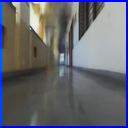} & \imgcell{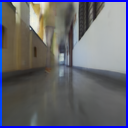} & \imgcell{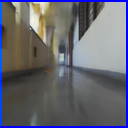} \\
&&&VANet&  \imgcell{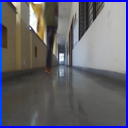}&\imgcell{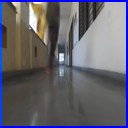} & \imgcell{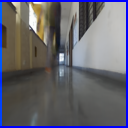} & \imgcell{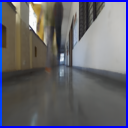} & \imgcell{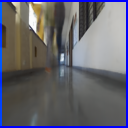} & \imgcell{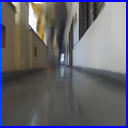} & \imgcell{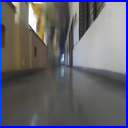} 

\end{tabular}}
\caption{Predictions on partially observable RoAM dataset by ACVG, ACVG-fa, ACPNet and VANet. The models were trained using 5 input-action frames to predict the next ten frames. During the inference phase, the predicted frames were increased to 15. In this case, the test sampling interval is two times the train sampling interval, i.e. $\Delta t_{\text{test}}=2 \times\Delta t_{\text{train}}$}
\label{fig:wacv_qual3}
\end{figure*}
% \textbf{Quantitative Evaluation:} 

% \textbf{Qualitative Evaluation:} Figure \ref{fig:wacv_qual}  $t=14$.

% \textbf{Discussion: } 

% \section{Conclusion }\label{sec:conclusion} A new video prediction framework capable of  generating multi-timestep future image frames in partially observable scenarios have been presented. Our initial quantitative and qualitative analysis showed promising results when we generated image frames conditioned on the action taken by the recording agent. 
