# Supplementary material for: Action-conditioned video data improves predictability
Source: arXiv:2404.05439 source file (2024-04-08)
Supplement: Supplementary file 2 [file supplimentry.tex]

% CVPR 2024 Paper Template; see https://github.com/cvpr-org/author-kit

\documentclass[10pt,twocolumn,letterpaper]{article}

%%%%%%%%% PAPER TYPE  - PLEASE UPDATE FOR FINAL VERSION
% \usepackage{cvpr}              % To produce the CAMERA-READY version
\usepackage[review]{cvpr}      % To produce the REVIEW version
% \usepackage[pagenumbers]{cvpr} % To force page numbers, e.g. for an arXiv version

% Import additional packages in the preamble file, before hyperref
\input{preamble}

% Include other packages here, before hyperref.
\usepackage{graphicx}
\usepackage{amsmath}
\usepackage{amssymb}
\usepackage{booktabs}
\usepackage{multicol}
\usepackage{array}
\usepackage{booktabs}
\usepackage{cite}
\usepackage[load-configurations=version-1]{siunitx}
% caption and subcaption work together
\usepackage{subcaption} % loads the caption package
\input{math_command.tex}
% It is strongly recommended to use hyperref, especially for the review version.
% hyperref with option pagebackref eases the reviewers' job.
% Please disable hyperref *only* if you encounter grave issues, e.g. with the
% file validation for the camera-ready version.
%
\newcommand{\imgcell}[1]{\includegraphics[scale=0.5]{#1}}
% If you comment hyperref and then uncomment it, you should delete
% ReviewTempalte.aux before re-running LaTeX.
% (Or just hit 'q' on the first LaTeX run, let it finish, and you
%  should be clear).
\usepackage[pagebackref,breaklinks,colorlinks]{hyperref}
\usepackage{subcaption} % loads the caption package

% Support for easy cross-referencing
\usepackage[capitalize]{cleveref}
\crefname{section}{Sec.}{Secs.}
\Crefname{section}{Section}{Sections}
\Crefname{table}{Table}{Tables}
\crefname{table}{Tab.}{Tabs.}

%%%%%%%%% PAPER ID  - \definecolor{cvprblue}{rgb}{0.21,0.49,0.74}
\usepackage[pagebackref,breaklinks,colorlinks,citecolor=cvprblue]{hyperref}

%%%%%%%%% PAPER ID  - PLEASE UPDATE
 % *** Enter the Paper ID here

\begin{document}

%%%%%%%%% TITLE - PLEASE UPDATE
\title{Action-conditioned video generation with new indoor robot motion dataset RoAM (supplementary)}

\author{First Author\\
Institution1\\
Institution1 address\\
{\tt\small firstauthor@i1.org}
% For a paper whose authors are all at the same institution,
% omit the following lines up until the closing ``}''.
% Additional authors and addresses can be added with ``\and'',
% just like the second author.
% To save space, use either the email address or home page, not both
\and
Second Author\\
Institution2\\
First line of institution2 address\\
{\tt\small secondauthor@i2.org}
}
\maketitle

%%%%%%%%% ABSTRACT

%%%%%%%%% BODY TEXT
\section{Adversarial Loss}
In addition to the reconstruction penalty discussed in \textit{Section 2.3: Loss and Training Loop}, we also use the adversarial loss given in \cite{mathieu}, \cite{villegas} and \cite{sarkar2021} to increase the sharpness of the generated images. In general, deterministic frameworks (like ACVG, ACPNet or MCNet) suffer from the averaging effects of the convolution operations and are compensated by adding the adversarial loss. The expression for the adversarial loss $\mathcal{L}_{adv}$ is similar to \cite{mathieu},:
\begin{equation}
 \mathcal{L}_{adv}=-\text{log}\sD([{x}_{-n+1:0},\tx_{1:T}]) \label{eq:L_adv}  
\end{equation}
where ${x}_{-n+1:0}$ is the sequence of n past input images,  $\tx_{1:T}$ represents the predicted future images by the generator of ACVG given by Eqs. (11) or (12) depending upon the generator or dual training phase of the network, and $\sD(.)$ is the output from the discriminator network. Let $x_{-n+1:T}$ be the concatenation of all $n+T$ ground truth images. The discriminator network is trained  on the loss function: 
\begin{equation}
    \mathcal{L}_{dis}=-\text{log}\sD(x_{-n+1:T})-\text{log}(1-\sD({x}_{-n+1:0},\tx_{1:T}))
\end{equation}
 The adversarial loss $\mathcal{L}_{adv}$ is scaled by a factor of $\mu $ before being added to the total reconstruction loss of the Generator Network given by Eqs. (20) and  (21) in the paper. The scaling factor $\mu$ is chosen to be much less than 1. In the case of RoAM dataset,  we choose $\mu=0.0001$.

 The architecture of the discriminator network is the same as given in \cite{sarkar2021}.
 
 \section{Additional Ablation Study Results }\label{sec:ablation}
 
 We have reported the $\text{L}_2$ norm error between the predicted normalised actuator action from the Actor network of ACVG to the ground truth values in \cref{fig:action1_error}. It can be seen here that the actor-network does a good job of predicting the actions as long as the predicted image frames from the Generator network are of decent accuracy. However, after $t>8$ timestep when the predicted image quality degrades, the error in the predicted actions by the Actor network also increases. This shows the other side of the dual dependency between the Generator and Actor network.
 We have included additional plots from the ablation study, which involved ACVG, ACVG-fa, ACPNet, and VANet. These plots, shown in Figs. \ref{fig:wacv_supply_abl1} and \ref{fig:wacv_supply_abl2}, pertain to a scenario where the train sampling interval $\Delta t_{\text{train}}$ is the same as the test sampling interval $\Delta t_{\text{test}}$.

In Figs. \ref{fig:roam_acvg_fa_vgg16} -   \ref{fig:roam_acvg_fa_psnr}, we provide plots for VGG16 cosine similarity, FVD score, SSIM, and PSNR indexes, respectively. Notably, the VGG cosine similarity plot in \cref{fig:roam_acvg_fa_vgg16} demonstrates that ACVG significantly outperforms the other three approaches. The FVD score of VANet is slightly higher than that of ACVG, but at the expense of a significantly larger parametric space, which is nearly 1.5 times that of ACVG. Previous work by Villegas et al. \cite{villegasNeurIPS2019} has already demonstrated that a larger parametric space can lead to more realistic image generation.

Nonetheless, when examining other quantitative plots in Figs. \ref{fig:roam_acvg_fa_vgg16}, \ref{fig:roam_acvg_fa_ssim}, and \ref{fig:roam_acvg_fa_psnr}, it becomes evident that ACVG outperforms VANet when it comes to approximating the dynamics of the scene and the objects in the  frame.

It is worth noting that at $t=0$ in \cref{fig:roam_acvg_fa_vgg16}, all three networks—ACVG, ACVG-fa, and VANet—begin at the same index. However, with larger time, ACVG-fa falls behind ACVG and exhibits a similar performance to ACPNet. This similarity arises because both ACVG-fa and ACPNet utilize a fixed augmented action state. Moreover, after $t=6$ in the plot, VANet's performance lags behind ACPNet, even though it has a much larger parametric space for approximating the spatio-temporal dynamics of the data. This further underscores our initial assertion that incorporating the action dynamics of the recording robot into the video prediction task is crucial in partially observable scenarios.
 \begin{figure}[t]
\centering
  \includegraphics[width=0.75\linewidth]{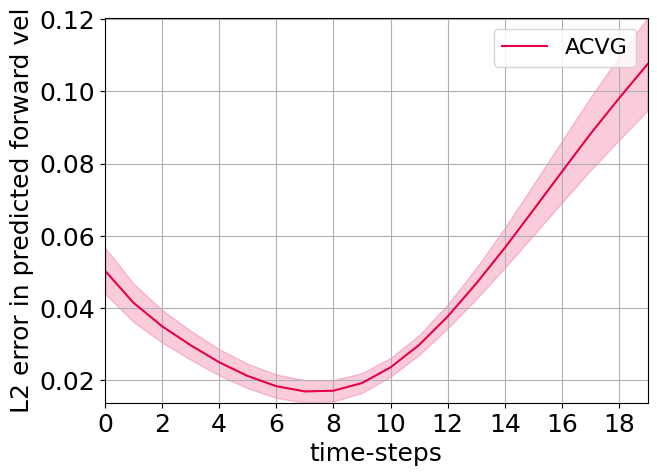}
  \caption{Plot of  $\text{L}_2$ error between the normalised actions predicted by the Actor-network of ACVG and the ground truth }
\label{fig:action1_error}
\end{figure}

 \begin{figure*}[ht]
\centering
\subcaptionbox{\label{fig:roam_acvg_fa_vgg16}}{\includegraphics[width=0.4\textwidth,height=4.5cm]{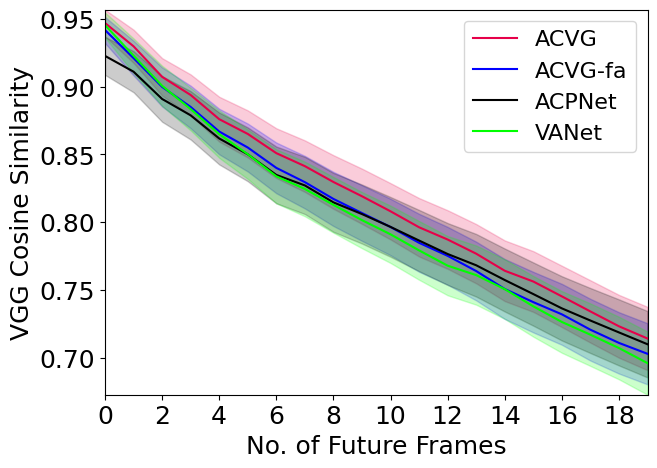}}%
 \hspace{2em}% <-- Seperation
\subcaptionbox{\label{fig:roam_acvg_fa_fvd}}{\includegraphics[width=0.4\textwidth, height=4.5cm]{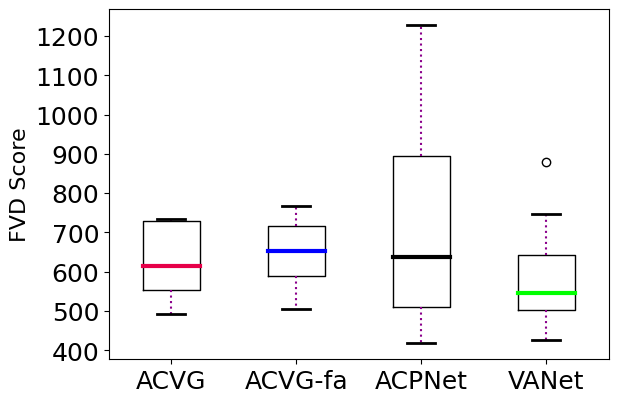}}
\hfill % <-- Seperation
\subcaptionbox{\label{fig:roam_acvg_fa_ssim}}{\includegraphics[width=0.4\textwidth, height=4.5cm]{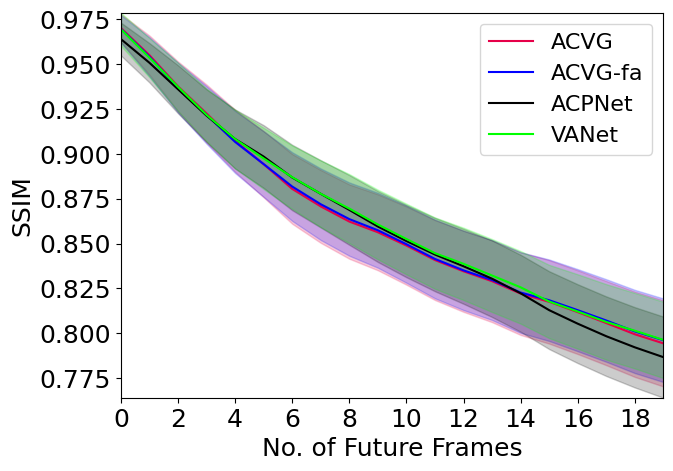}}%
 \hspace{2em}% <-- Seperation
\subcaptionbox{\label{fig:roam_acvg_fa_psnr}}{\includegraphics[width=0.4\textwidth, height=4.5cm]{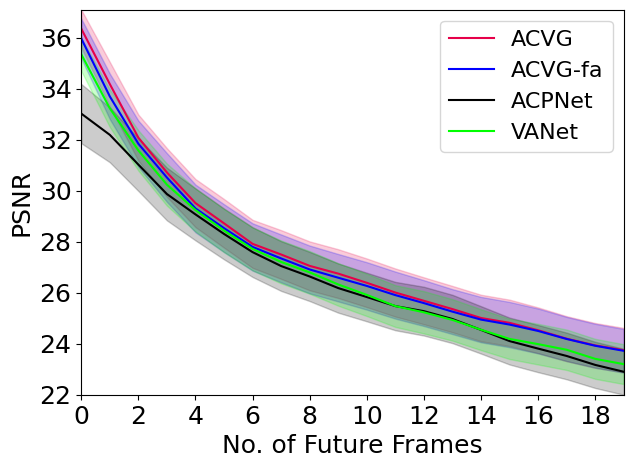}}%
\caption{A frame-wise ablation study with quantitative analysis of  ACVG, ACVG-fa, ACPNet and VANet on RoAM dataset. (a) VGG 16 Cosine Similarity (\textbf{higher is better}) (b) FVD score (\textbf{lower is better}) (c)  SSIM (\textbf{higher is better}) and  (d) PSNR index (\textbf{higher is better}), are shown  for predicting 20 frames into the future from past 5 frames. Here the sampling interval between train and test time is the same. }
\label{fig:wacv_supply_abl1}
\end{figure*}

In Fig \ref{fig:wacv_supply_abl2} we provided the additional ablation study plots for the second scenario where the sampling interval at test time $\Delta t_{\text{test}}$ is twice the sampling interval at train time $\Delta t_{\text{train}}$. This makes the objects in the image frame move faster relative to the ones that were used during the training phase. In Figs. \ref{fig:roam_acvg_half_vgg16} -   \ref{fig:roam_acvg_half_psnr}, we report VGG16 cosine similarity, FVD score, SSIM, and PSNR indexes, respectively. From the plots in \cref{fig:wacv_supply_abl2} it is evident that learning the dual interplay of dynamics between the action and observed image data pays off in the long run as the same can be inferred from \cref{fig:roam_acvg_half_vgg16}. It can be seen from  Figs. \ref{fig:roam_acvg_fa_psnr} and \ref{fig:roam_acvg_half_psnr} that both the ACVG and ACVG-fa follow almost indistinguishable trajectories in both cases. This is due to the fact that ACVG and ACVG-fa have the same Generator network architecture, and thus have similar noise profiles. 

We have also provided the larger version of the Quantitative analysis plots given in Fig. 4 of the paper here in \cref{fig:wacv_quant}.
We have provided additional qualitative raw image frames from ACVG, ACVG-fa, ACPNet, and VANet in Figs. \ref{fig:wacv_qual1}, \ref{fig:wacv_qual2}, and \ref{fig:wacv_qual3}. In \cref{fig:wacv_qual3}, where the test sampling time interval is twice the training data sampling interval, it is evident that all four networks underestimate human motion. This is expected because at $\Delta t_{\text{test}}=2 \times\Delta t_{\text{train}}$, all objects appear to move much faster than what these frameworks have learned to anticipate. However, ACVG performs reasonably well in this scenario.

At time step $t=19$ in \cref{fig:wacv_qual3}, it might seem that ACPNet performs similarly to ACVG. However, a closer examination reveals that the image frame generated by ACPNet at $t=19$ exhibits multiple artifacts compared to ACVG. The most significant difference in the predicted image frames among the four frameworks is noticeable in the time-stamped frames in \cref{fig:wacv_qual2}. Here, at $t=21$, only ACVG effectively predicts the silhouette of the moving human figure, while ACPNet and VANet overestimate the human motion and predict that the human has already moved out of the frame.

The codes for the implementation ACVG can be found in \url{https://github.com/WACV-paper-702/ACVG-wacv2024.git}
\begin{figure*}[ht]
\centering
\subcaptionbox{\label{fig:roam_acvg_half_vgg16}}{\includegraphics[width=0.4\textwidth,height=4.5cm]{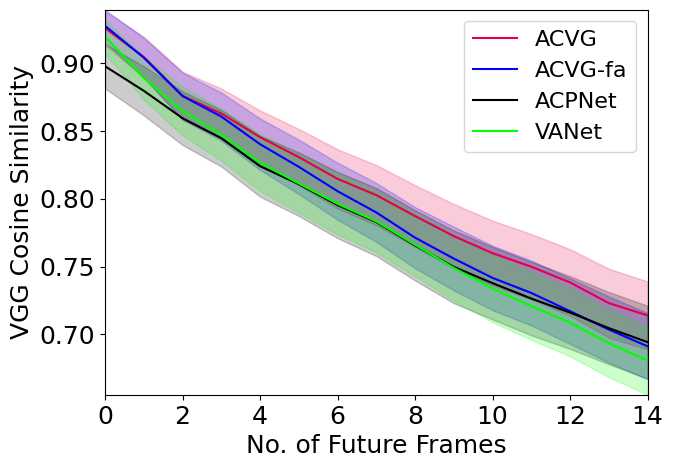}}%
 \hspace{2em}% <-- Seperation
\subcaptionbox{\label{fig:roam_acvg_half_fvd}}{\includegraphics[width=0.4\textwidth, height=4.5cm]{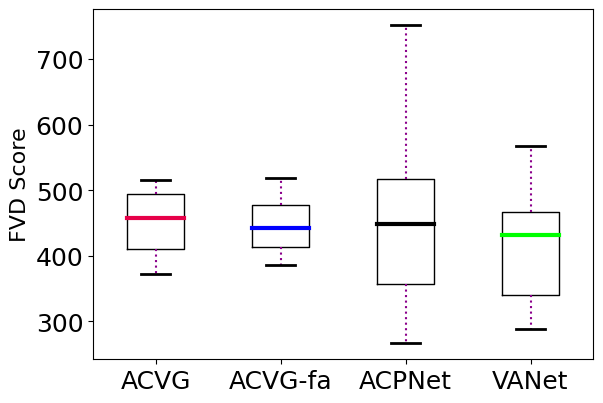}}
\hfill % <-- Seperation
\subcaptionbox{\label{fig:roam_acvg_half_ssim}}{\includegraphics[width=0.4\textwidth, height=4.5cm]{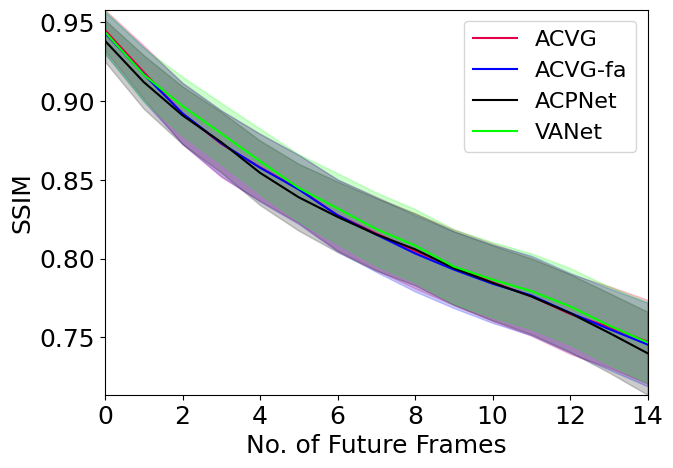}}%
 \hspace{2em}% <-- Seperation
\subcaptionbox{\label{fig:roam_acvg_half_psnr}}{\includegraphics[width=0.4\textwidth, height=4.5cm]{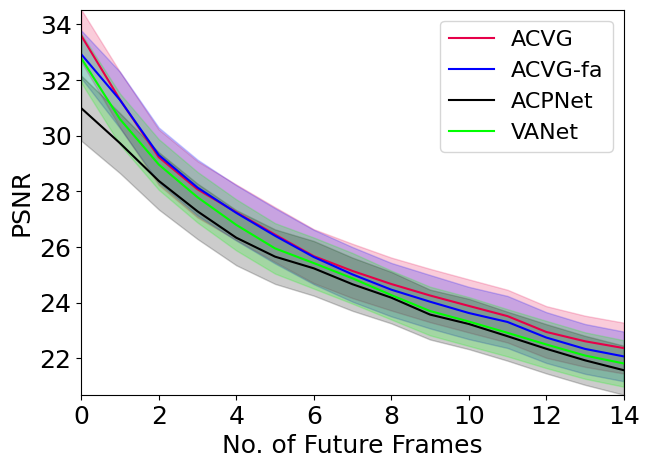}}%
\caption{A Frame-wise ablation study with quantitative analysis of  ACVG, ACVG-fa, ACPNet and VANet on RoAM dataset. (a) VGG 16 Cosine Similarity (\textbf{higher is better}) (b) FVD score (\textbf{lower is better}) (c)  SSIM (\textbf{higher is better}) and (d)  PSNR index (\textbf{higher is better}), are shown  for predicting 15 frames into the future from past 5 frames. Here the sampling interval at test time $\Delta t_{\text{test}}$ is twice the sampling interval at train time $\Delta t_{\text{train}}$. }
\label{fig:wacv_supply_abl2}
\end{figure*}

\begin{figure*}[ht]
\centering
\subcaptionbox{\label{fig:roam_quant_vgg16}}{\includegraphics[width=0.4\textwidth]{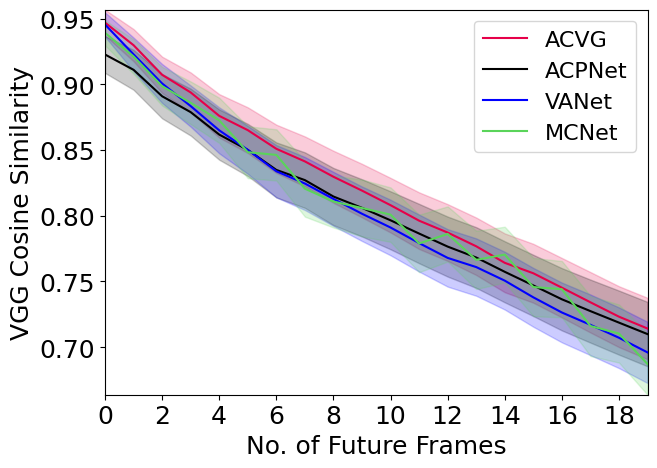}}%
 \hspace{2em}% <-- Seperation
\subcaptionbox{\label{fig:roam_quant_fvd}}{\includegraphics[width=0.4\textwidth]{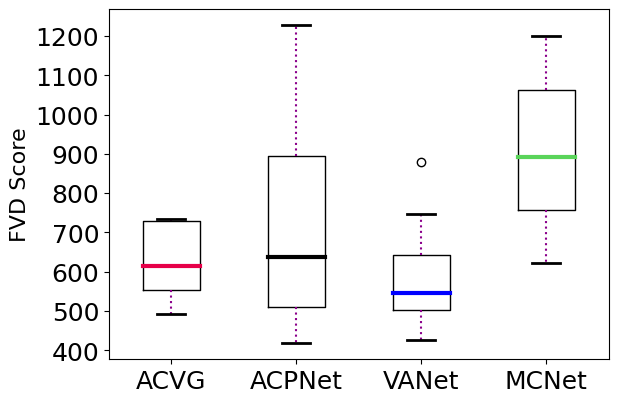}}
\hfill % <-- Seperation
\subcaptionbox{\label{fig:roam_quant_ssim}}{\includegraphics[width=0.4\textwidth]{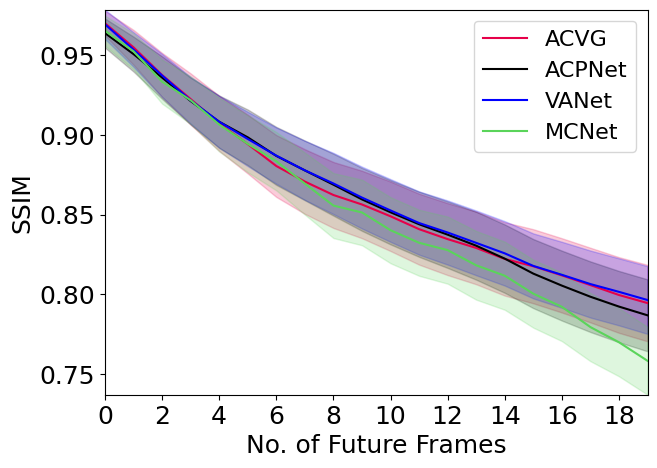}}%
 \hspace{2em}% <-- Seperation
\subcaptionbox{\label{fig:roam_quant_psnr}}{\includegraphics[width=0.4\textwidth]{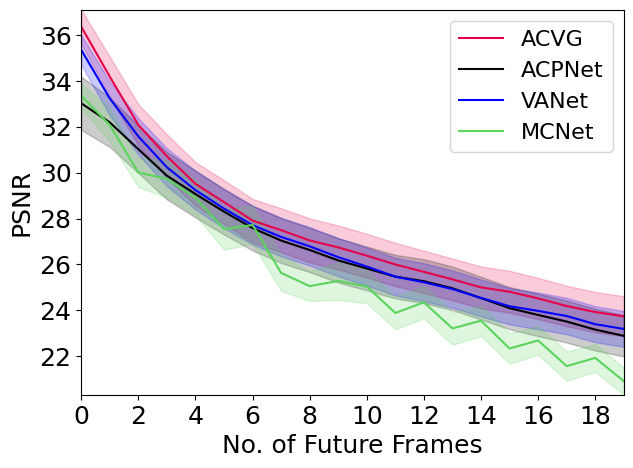}}%
\caption{A Frame-wise quantitative analysis of   ACVG, ACPNet,VANet and MCNet on RoAM dataset for predicting 20 frames into the future based on the past history of 5 frames. We have plotted the mean performance index for (a) VGG 16 Cosine Similarity (\textbf{higher is better}), (b) FVD score (\textbf{lower is better}), (c) SSIM (\textbf{higher is better}), and (d) PSNR (\textbf{higher is better}) on the test set. }
\label{fig:wacv_quant}
\end{figure*}

\begin{figure*}[ht]
\resizebox{\textwidth}{!}{\begin{tabular}{cccccccccccc}
 & t=1 & t=3 & t=5 & t=6 & t=7 & t=9 & t=13 & t=15 & t=17 & t=21\\
Ground Truth & \imgcell{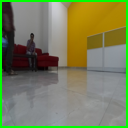} & \imgcell{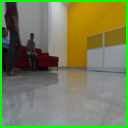} & \imgcell{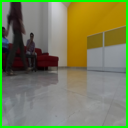}&  \imgcell{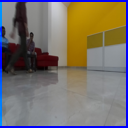}&\imgcell{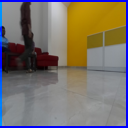} & \imgcell{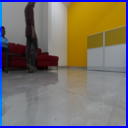} & \imgcell{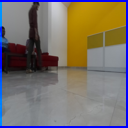} & \imgcell{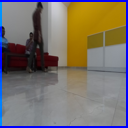} & \imgcell{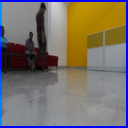} & \imgcell{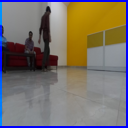} \\
&&&ACVG&  \imgcell{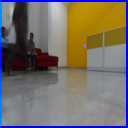}&\imgcell{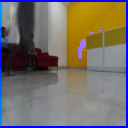} & \imgcell{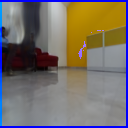} & \imgcell{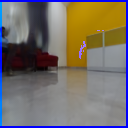} & \imgcell{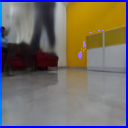} & \imgcell{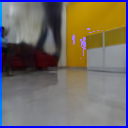} & \imgcell{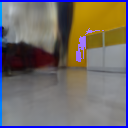} \\
&&&ACPNet&  \imgcell{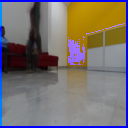}&\imgcell{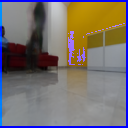} & \imgcell{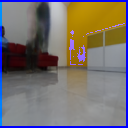} & \imgcell{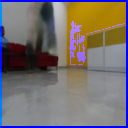} & \imgcell{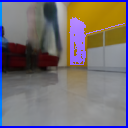} & \imgcell{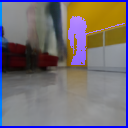} & \imgcell{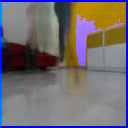} \\
&&&VANet&  \imgcell{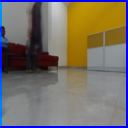}&\imgcell{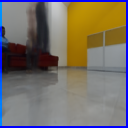} & \imgcell{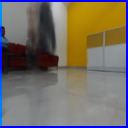} & \imgcell{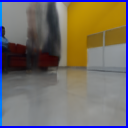} & \imgcell{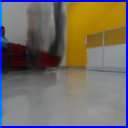} & \imgcell{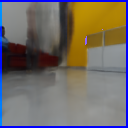} & \imgcell{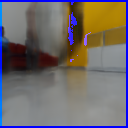} \\
&&&MCNet&  \imgcell{qual_results/mcnet/pred_0006.png}&\imgcell{qual_results/mcnet/pred_0008.png} & \imgcell{qual_results/mcnet/pred_0010.png} & \imgcell{qual_results/mcnet/pred_0012.png} & \imgcell{qual_results/mcnet/pred_0014.png} & \imgcell{qual_results/mcnet/pred_0016.png} & \imgcell{qual_results/mcnet/pred_0020.png}
\end{tabular}}
\caption{Predictions on partially observable RoAM dataset by ACVG, ACPNet, VANet, and MCNet. The models were trained using 5 input-action frames to predict the next ten frames. During the inference phase, the predicted frames were increased to 20}
\label{fig:wacv_qual1}
\end{figure*}

\begin{figure*}[ht]
\resizebox{\textwidth}{!}{\begin{tabular}{cccccccccccc}
 & t=1 & t=3 & t=5 & t=7 & t=9 & t=11 & t=13 & t=15 & t=17 & t=21\\
Ground Truth & \imgcell{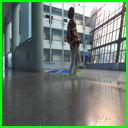} & \imgcell{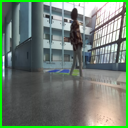} & \imgcell{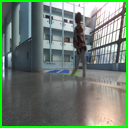}&  \imgcell{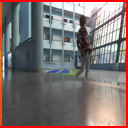}&\imgcell{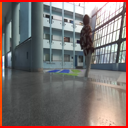} & \imgcell{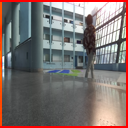} & \imgcell{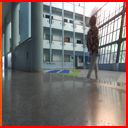} & \imgcell{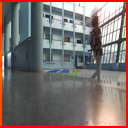} & \imgcell{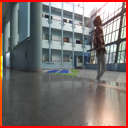} & \imgcell{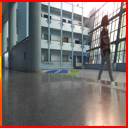} \\
&&&ACVG&  \imgcell{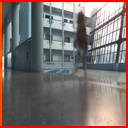}&\imgcell{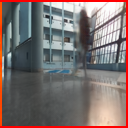} & \imgcell{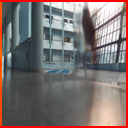} & \imgcell{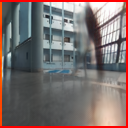} & \imgcell{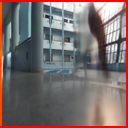} & \imgcell{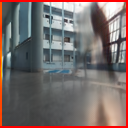} & \imgcell{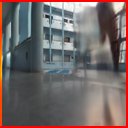} \\
&&&ACVG-fa&  \imgcell{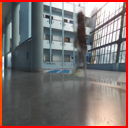}&\imgcell{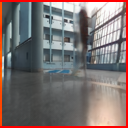} & \imgcell{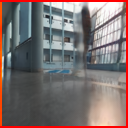} & \imgcell{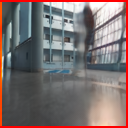} & \imgcell{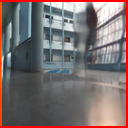} & \imgcell{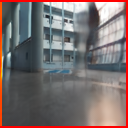} & \imgcell{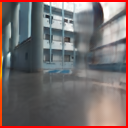}\\
&&&ACPNet&  \imgcell{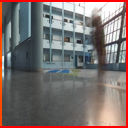}&\imgcell{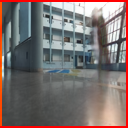} & \imgcell{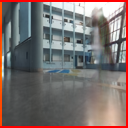} & \imgcell{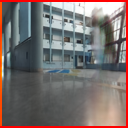} & \imgcell{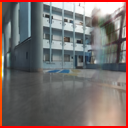} & \imgcell{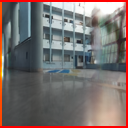} & \imgcell{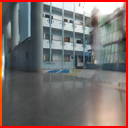} \\
&&&VANet&  \imgcell{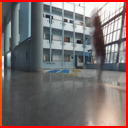}&\imgcell{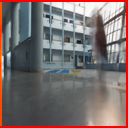} & \imgcell{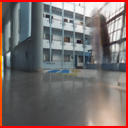} & \imgcell{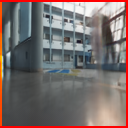} & \imgcell{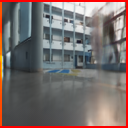} & \imgcell{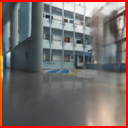} & \imgcell{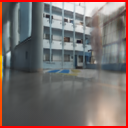} 

\end{tabular}}
\caption{Predictions on partially observable RoAM dataset by ACVG, ACVG-fa, ACPNet and VANet. The models were trained using 5 input-action frames to predict the next ten frames. During the inference phase, the predicted frames were increased to 20. In this case the test sampling interval is the same as the train sampling interval, i.e. $\Delta t_{\text{test}}=\Delta t_{\text{train}}$}
\label{fig:wacv_qual2}
\end{figure*}

\begin{figure*}[ht]
\resizebox{\textwidth}{!}{\begin{tabular}{cccccccccccc}
 & t=1 & t=3 & t=5 & t=7 & t=9 & t=11 & t=13 & t=15 & t=17 & t=19\\
Ground Truth & \imgcell{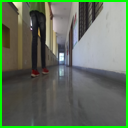} & \imgcell{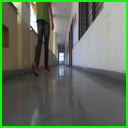} & \imgcell{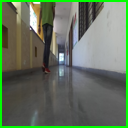}&  \imgcell{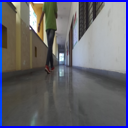}&\imgcell{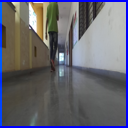} & \imgcell{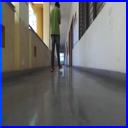} & \imgcell{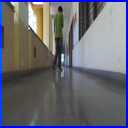} & \imgcell{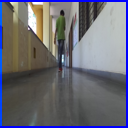} & \imgcell{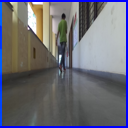} & \imgcell{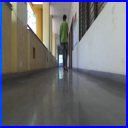} \\
&&&ACVG&  \imgcell{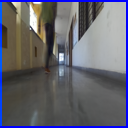}&\imgcell{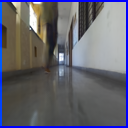} & \imgcell{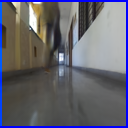} & \imgcell{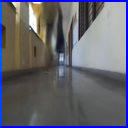} & \imgcell{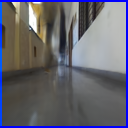} & \imgcell{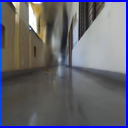} & \imgcell{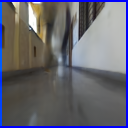} \\
&&&ACVG-fa&  \imgcell{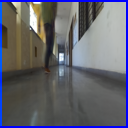}&\imgcell{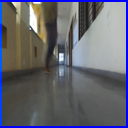} & \imgcell{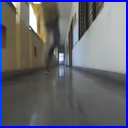} & \imgcell{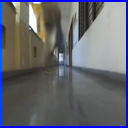} & \imgcell{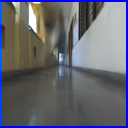} & \imgcell{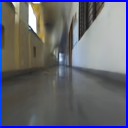} & \imgcell{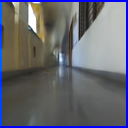}\\
&&&ACPNet&  \imgcell{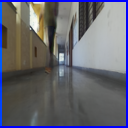}&\imgcell{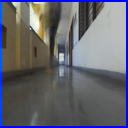} & \imgcell{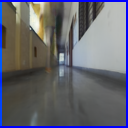} & \imgcell{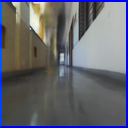} & \imgcell{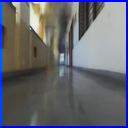} & \imgcell{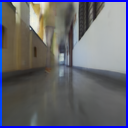} & \imgcell{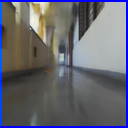} \\
&&&VANet&  \imgcell{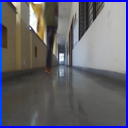}&\imgcell{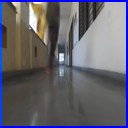} & \imgcell{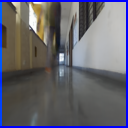} & \imgcell{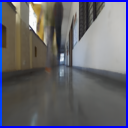} & \imgcell{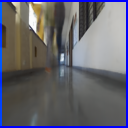} & \imgcell{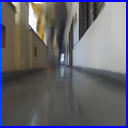} & \imgcell{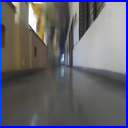} 

\end{tabular}}
\caption{Predictions on partially observable RoAM dataset by ACVG, ACVG-fa, ACPNet and VANet. The models were trained using 5 input-action frames to predict the next ten frames. During the inference phase, the predicted frames were increased to 15. In this case, the test sampling interval is two times the train sampling interval, i.e. $\Delta t_{\text{test}}=2 \times\Delta t_{\text{train}}$}
\label{fig:wacv_qual3}
\end{figure*}
% \textbf{Quantitative Evaluation:} 

% \textbf{Qualitative Evaluation:} Figure \ref{fig:wacv_qual}  $t=14$.

% \textbf{Discussion: } 

% \section{Conclusion }\label{sec:conclusion} A new video prediction framework capable of  generating multi-timestep future image frames in partially observable scenarios have been presented. Our initial quantitative and qualitative analysis showed promising results when we generated image frames conditioned on the action taken by the recording agent. 

%%%%%%%%% REFERENCES
{\small
\bibliographystyle{ieee_fullname}
\bibliography{egbib}
}

\end{document}
